# Supplementary material for: Infrared phonons as a probe of a spin-liquid states in herbertsmithite ZnCu3(OH)6Cl2
Source: arXiv:1608.01240 source file (2017-01-23)
Supplement: Supplementary file 1 [file HS_Suppl_v01_subm.pdf]

# SUPPLEMENTAL MATERIAL

# Infrared phonons as a probe of a spin-liquid states in herbertsmithite $ZnCu_3(OH)_6Cl_2$

A. B. Sushkov,[1] G. S. Jenkins,[1] Tian-Heng Han,[2] Young Lee,[3] and H. D. Drew[1]

[1]*Center for Nanophysics and Advanced Materials, Department of Physics, University of Maryland, College Park, Maryland 20742, USA*

[2]*University of Chicago, Chicago, IL, USA*

[3]*Massachusetts Institute of Technology, Cambridge, MA, USA*

In this Supplemental part, we show reflectivity spectra and fit parameters of extra phonons electric dipole active in kagome plane ($e||ab$) and of phonons active in $e||c$ polarization.

## I. EXTRA PHONON MODES IN $e||ab$ POLARIZATION

Figure 1 shows data for the vicinity of $a8$ phonon. Both modes harden upon cooling, keep their spectral weight constant, and they both have quite high scattering rate $\gamma$ which is constant with temperature. Such independence on temperature of the $\gamma$ parameter may be caused by structural disorder and by magneto-elastic disorder where the elastic constants of certain bonds depend on mutual orientation of spins. Figure 2 shows data for one extra

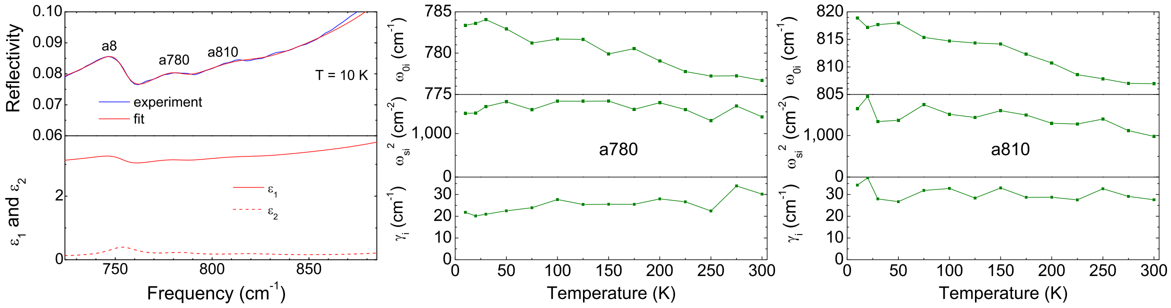


FIG. 1. (Color online). Reflectivity, dielectric function, and fit parameters of the Lorentzian model (Eq. (1) of the paper) for two extra phonons near $a8$ phonon.

phonon $a980$ near $a9$ phonon. Fit model does not reproduce well the shape of $a980$ phonon which usually happens when the frequency of weak phonon is in the minimum of reflectivity of strong phonon. Fit parameter $\gamma$ is growing toward zero temperature but we will cannot draw any conclusion from these data because of the quality of the fit.

Figure 3 shows data for two extra phonons near $a10$ phonon. At such high frequencies, phonons modes consist mostly of hydrogen atoms motions. Without ab initio or shell model calculations of phonons, we don't know how many hydrogen dominated phonon modes should be in this crystal. Two modes $a3325$ and $a3438$ show classical temperature behavior of the $\gamma$ parameter. This means that there is no much of disorder both of crystalline and magnetic origin.

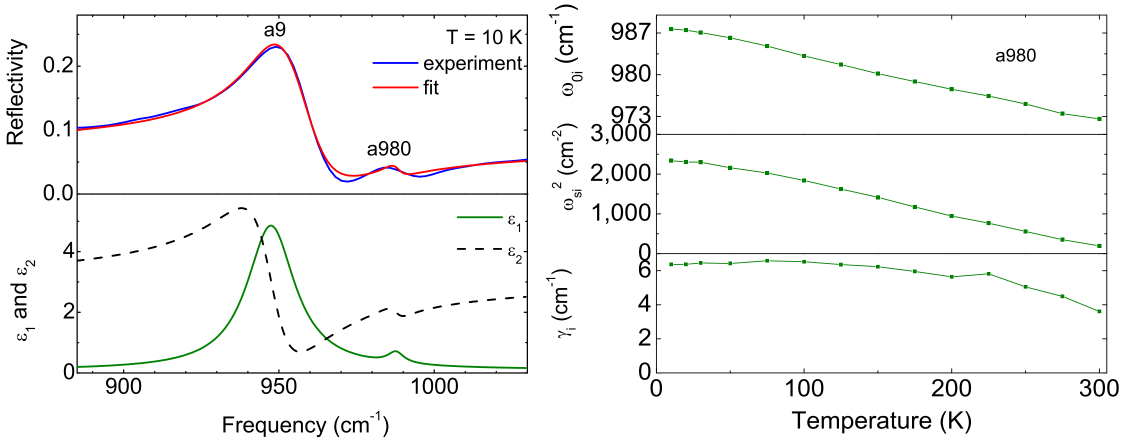


FIG. 2. (Color online). Reflectivity, dielectric function and fit parameters of the Lorentzian model (Eq. (1) of the paper) for an extra phonon near $a9$ phonon.

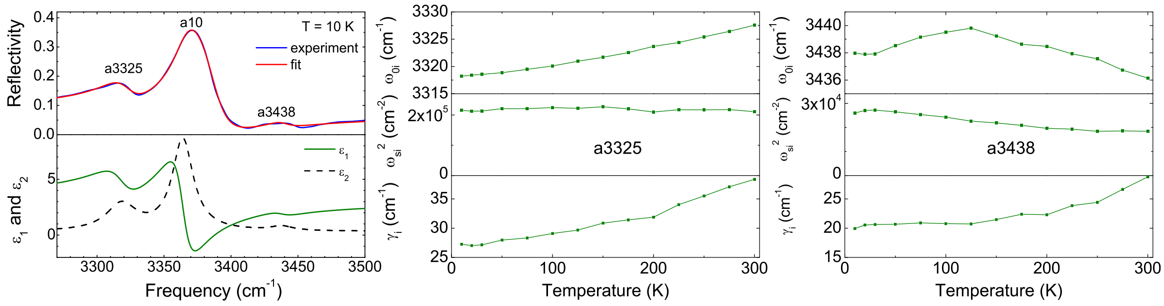


FIG. 3. (Color online). Reflectivity, dielectric function and fit parameters of the Lorentzian model (Eq. (1) of the paper) for two extra phonons near $a10$ phonon.

## II. EXTRA PHONON MODES IN $e||c$ POLARIZATION

Figure 4 shows data for the vicinity of $c6$ phonon. These phonons demonstrate quite standard temperature behavior except softening of the $c600$ mode. In principle, phonon softening may be due to the spin-phonon coupling effect but also can be purely structural.

Figure 5 shows data for the vicinity of $c7$ phonon. A striking feature of these hydrogen dominated phonons is linear with temperature softening of five out of six modes. Again, a theoretical study is needed to understand the origin of such phonon softening.

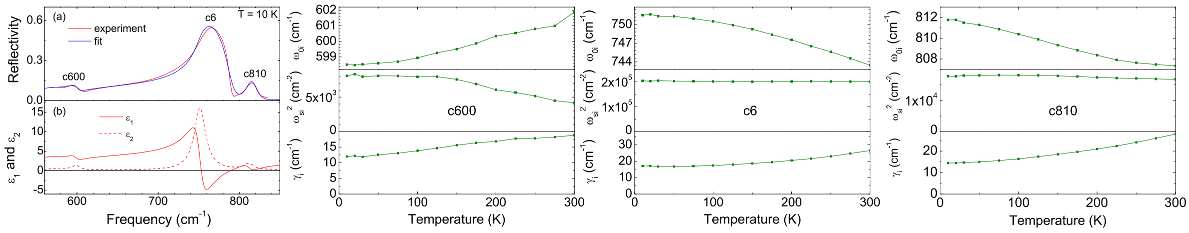


FIG. 4. (Color online). Reflectivity, dielectric function and fit parameters of the Lorentzian model (Eq. (1) of the paper) for two extra phonons near $c6$ phonon.

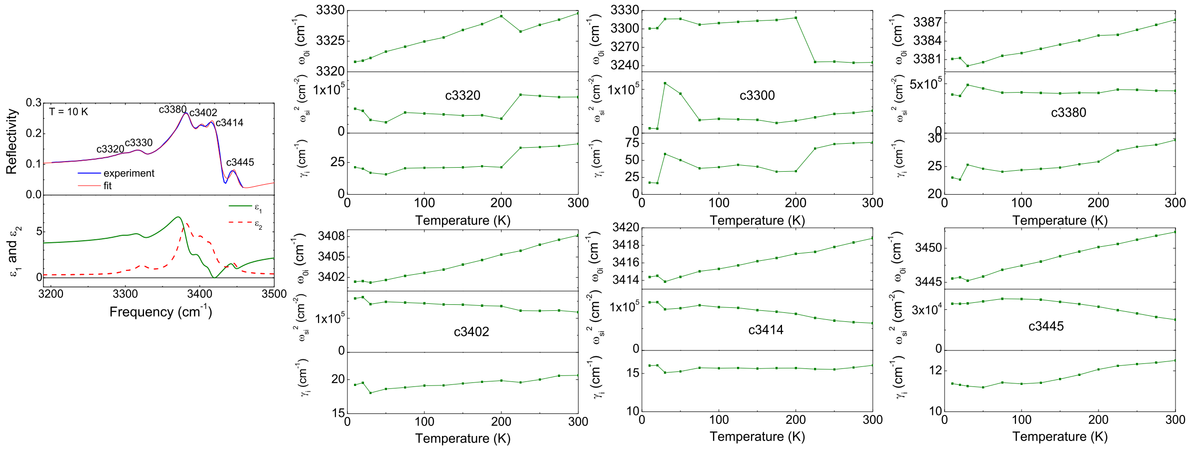


FIG. 5. (Color online). Reflectivity, dielectric function and fit parameters of the Lorentzian model (Eq. (1) of the paper) for two extra phonons near $c7$ phonon.
